# Supplementary material for: Cooperation Does Matter: Exploring Multi-Order Bilateral Relations for Audio-Visual Segmentation
Source: arXiv:2312.06462 source file (2024-04-07)
Supplement: Supplementary file 1 [file supp2_fig_architecture.tex]

\begin{figure*}[t!]
    \centering
    \includegraphics[width=2.0\columnwidth]{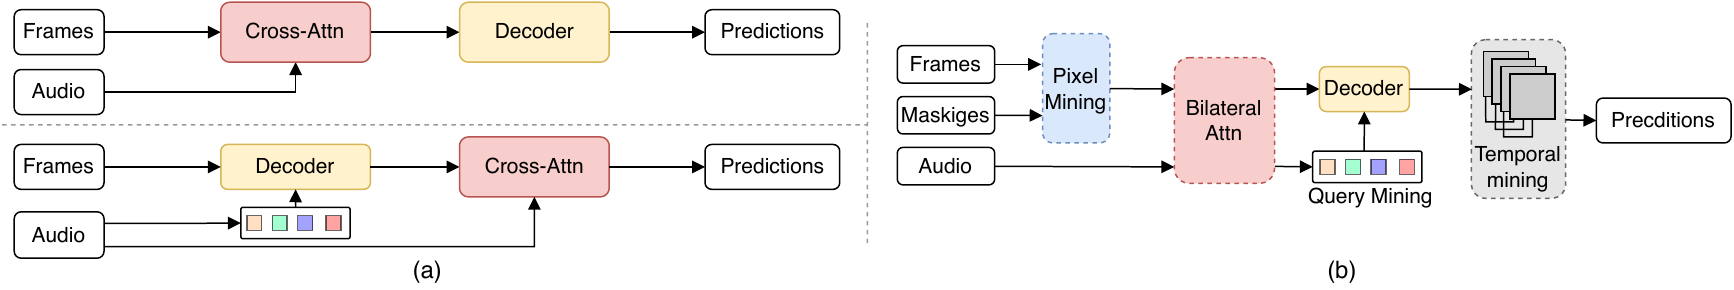}
    % \vspace{-0.2cm}
    \caption{
    Framework comparison between the existing mainstream methods~\cite{2022AVS,2023avsegformer,ling2023hear} and our proposed COMBO.
    (a) The framework of the mainstream approaches, which mainly explores the stage of the fusion.
    (b) Our COMBO framework, which simultaneously explores multi-order relations.
    } 
    \label{fig:supp_figure2_architecture}
    % \vspace{-0.5cm}
\end{figure*}
