# Supplementary material for: Cooperation Does Matter: Exploring Multi-Order Bilateral Relations for Audio-Visual Segmentation
Source: arXiv:2312.06462 source file (2024-04-07)
Supplement: Supplementary file 2 [file ablation_appendix.tex]

\begin{table}[t!]
    \centering
    \setlength{\tabcolsep}{5pt} % adjust column spacing
     % adjust row spacing
    \begin{adjustbox}{max width=0.8\linewidth}
    \begin{tabular}{cccccc} 
        \toprule 
         \multirow{2}*{Proposal Generator}  & \multicolumn{2}{c}{\textbf{S4}}  & \multicolumn{2}{c}{\textbf{AVSS}} \\
        \cmidrule(lr){2-3}  \cmidrule(lr){4-5}  
         & $\mathcal{M_J}$ & $\mathcal{M_F}$ & $\mathcal{M_J}$ & $\mathcal{M_F}$  \\
        \midrule
         & 80.6 &  89.6  &\\ 
         Segment-Anything~\cite{2023_SAM_ICCV}  & -  &  - &   \\
         Mobile-SAM~\cite{2023_mobile_sam}  & \checkmark  &  - &   \\
         Semantic-SAM~\cite{2023_semanticsam}  &  81.7 & 90.1  & 33.3 & 37.3  \\
        \bottomrule 
    \end{tabular}
    \end{adjustbox}
    \captionsetup{justification=raggedright}
    \caption{Quantitative comparison results of different methods on AVSBench-semantic~(audio-visua semantic segmentation,~AVSS).}

    \label{tab:exp_ablation_all}
\end{table}
% 这个表格，放到appendix里面？
% No sam  OrderedDict([('sem_seg', {'mIoU': 0.8084, 'f_score': 0.9001})])
